# Supplementary material for: Online Scheduling via Gradient Descent for Weighted Flow Time Minimization
Source: arXiv:2409.03020 source file (2024-09-04)
Supplement: Supplementary file 1 [file 10.appendix.tex]

\section{Appendix}

\begin{lemma}
    \label{lem:unrelated-GD-decrease}
    For unweighted unrelated machine scheduling, consider the residual objective function $f(\bx)$. Then, GD decreases $f(\bx)$ most against arbitrary scheduling.
\end{lemma}
\begin{proof}
    Let the alive job set of $\bx$ be $J$. Consider the optimal assignment of $\bx$. In the unweighted unrelated machine scheduling, the assignment forms a matching from job to machine. Let $J_i$ denotes the job set in machine $i$ in the optimal assignment. 
    
    Now, consider arbitrary scheduling $\pi: [M] \to [N]$, i.e., $\pi(i)=j$ denotes processing job $j$ on the machine $i$. Focus on $\pi(i) = j$. Let $GD_i$ denotes the rate of decreasing $f(\bx)$ for GD algorithm on the machine $i$, which is $|J_i|$. Then, we define $S_i$ analogously for the scheduling $\pi$. w.r.t the machine $i$. Next, we will show $GD_i$ always decreases $f(\bx)$ more than $S_i$ does which is $GD_i \geq S_i$ by the following two cases. If $j \in J_i$, clearly $S_i \leq |J_i|$ because $j$ decreases $f(\bx)$ at the rate of the number of jobs behind it in $J_i$. Thus, $S_i \leq GD_i$. We only need to consider $j \in J_{i'}$ and $i' \neq i$. Similarly, job $j$ decreases $f(\bx)$ at the rate of the number of jobs behind it in $J_{i'}$ which is $|J_{i'}^{>j}| \frac{p_{i'j}}{p_{ij}}$. Here, $p_{ij}$ is the processing time of job $j$ on the machine $i$ and $|J_i^{>j}|$ is the number of jobs behind job $j$ in $J_i$. Suppose that moving job $j$ from $i'$ to $i$. Let $\Delta_i$ denotes the change of the total completion time due to the move. Then, we have 
    $$ \Delta_i = p_{i,\leq j} + |J_{i}^{>j}| p_{ij}$$
    and 
    $$ \Delta_{i'} = p_{i', \leq j} + |J_{i'}^{>j}| p_{i' j}$$
    where $p_{i,\leq j} = \sum_{j' \in J_i, p_{ij'} \leq p_{ij}} p_{ij'}$. Due to the optimality, we know $\Delta_i \geq \Delta_{i'}$. 
    
    Now we shift to bound $\frac{p_{i,\leq j}}{p_{ij}}$. Because $p_{i,\leq j} \leq |J_i^{\leq j}|p_{ij}$, $\frac{p_{i,\leq j}}{p_{ij}} \leq |J_i^{\leq j}|$. Thus, we have 
    $$ S_i = |J_{i'}^{>j}| \frac{p_{i'j}}{p_{ij}} \leq \frac{\Delta_{i'}}{p_{ij}} \leq \frac{\Delta_{i}}{p_{ij}} =  \frac{p_{i,\leq j} + |J_{i}^{>j}| p_{ij}}{p_{ij}} \leq |J_i^{\leq j}| + |J_{i}^{>j}| = |J_i| = GD_i$$
    Therefore, we have the lemma~\ref{lem:unrelated-GD-decrease}.
\end{proof}

\subsection{Weighted Non-Clairvoyant LS}

In this section, all $x$ are between $0$ and $1$.

$v(x) = - \sum_{i < j \in [n]} x_i x_j \min\{p_i w_j, p_j w_i\} - \frac{1}{2} \sum_{i \in [n]} x_i x_i w_i p_i + \sum_{i \in [n]} (M - \frac{1}{2} w_i p_i) x_i$

\begin{lemma} [Theorem 10 in \cite{ReiGP02}]
    \label{lem:check-GS}
    Consider any function $v: \set{0,1}^N \to \R_+$. If $v$ is submodular, then $v$ is gross substitutes if and only if 
    $$ v(S \cup \set{a, b}) + v(S \cup \set{c}) \leq \max\set{v(S \cup \set{a, c}) + v(S \cup \set{b}), v(S \cup \set{b, c}) + v(S \cup \set{a})}$$
    for every $S \cup \set{a, b, c} \subseteq N$.
\end{lemma}

\begin{lemma}
    For $\eps \in 1 / \Z_+$, let $\Tv^{+\eps}: \{0,1\}^{N := [\sum_{i\in [n]} p_i/ \eps]} \to \R_+$ specified by
    \begin{align*}
        \Tv^{+\eps}(\set{\Tx_{i,1}, ..., \Tx_{i, p_i / \eps}}_{i \in [n]}) &= -\eps^2 \left( \sum_{\substack{i < i' \in [n] \\j \in [ p_i / \eps] \\ j' \in [p_{i'} / \eps]}} \Tx_{i,j} \Tx_{i', j'}\min\set{\frac{w_i}{p_i}, \frac{w_{i'}}{p_{i'}}} \right) \\
        &-\eps^2\left(\frac{1}{2}\sum_{i \in [n]} (\sum_{j \in [p_i / \eps]} \Tx_{i,j})(\sum_{j' \in [p_i / \eps]} \Tx_{i,j'}) \frac{w_i}{p_i} \right) \\
        &+ \eps \sum_{i\in [n]} (\frac{M}{p_i} - \frac{1}{2} w_i) \sum_{j \in [p_i / \eps]} \Tx_{i,j}
    \end{align*} 
    Then, $\Tv^{+\eps}$ is gross substitutes.
\end{lemma}
\begin{proof}
    Clearly, $\Tv^{+\eps}$ is submodular. For brevity, we drop $+\eps$ from the notation. Due to Lemma~\ref{lem:check-GS}, we only need to check 
    $$ \Tv(S \cup \set{a, b}) + \Tv(S \cup \set{c}) \leq \max\set{\Tv(S \cup \set{a, c}) + \Tv(S \cup \set{b}), \Tv(S \cup \set{b, c}) + \Tv(S \cup \set{a})}$$
    for every $S \subseteq N$ and $a,b,c \in N$. Let $X(a)$ be the corresponding $\Tx_{i,j} \in N$ and $I(a)$ be the corresponding $i$. Remark that $X(s)$ is $1$ for $s \in S \cup \set{a, b, c}$. We can decompose $\Tv(S \cup \set{a, b})$ as 
    \begin{align*}
        \Tv(S \cup \set{a, b}) &= -\eps^2 \left( \sum_{s \in S} X(s) X(a) \min\{\frac{w_{I(s)}}{p_{I(s)}}, \frac{w_{I(a)}}{p_{I(a)}}\} + \sum_{s \in S} X(s) X(b) \min\{\frac{w_{I(s)}}{p_{I(s)}}, \frac{w_{I(b)}}{p_{I(b)}}\} \right) \\  
        & -\eps^2 X(a) X(b) \min\{\frac{w_{I(a)}}{p_{I(a)}}, \frac{w_{I(b)}}{p_{I(b)}}\} \\
        & +\eps \sum_{s \in S \cup \set{a, b}} (M - \frac{1}{2} \frac{w_{I(s)}}{p_{I(s)}})X(s)
    \end{align*}
    Similarly, we can rewrite $\Tv(S \cup \set{a})$ as 
    \begin{align*}
        \Tv(S \cup \set{a}) = -\eps^2 \left( \sum_{s \in S} X(s) X(a) \min\{\frac{w_{I(s)}}{p_{I(s)}}, \frac{w_{I(a)}}{p_{I(a)}}\right)+\eps \sum_{s \in S \cup \set{a}} (M - \frac{1}{2} \frac{w_{I(s)}}{p_{I(s)}})X(s)
    \end{align*}
    Then, it is equivalent to show the following inequality
    $$ -\min\{\frac{w_{I(a)}}{p_{I(a)}}, \frac{w_{I(b)}}{p_{I(b)}}\} \leq \max\set{-\min\{\frac{w_{I(a)}}{p_{I(a)}}, \frac{w_{I(c)}}{p_{I(c)}}\}, -\min\{\frac{w_{I(b)}}{p_{I(b)}}, \frac{w_{I(c)}}{p_{I(c)}}\}}$$
    which is true by simple rearranging
    $$  \max\{-\frac{w_{I(a)}}{p_{I(a)}}, -\frac{w_{I(b)}}{p_{I(b)}}\} \leq \max\set{\max\{-\frac{w_{I(a)}}{p_{I(a)}}, -\frac{w_{I(c)}}{p_{I(c)}}\}, \max\{-\frac{w_{I(b)}}{p_{I(b)}}, -\frac{w_{I(c)}}{p_{I(c)}}\}}$$
    Therefore, we have the lemma.
\end{proof}

Let $\bone_{n}^m$ be a vector with $n$ entries and first $m$ entries are $1$.

\begin{lemma}
    Let $v^{+} : \Q_{[0,1]}^n \to \R_+$ specified by 
    %$$ v^{+}(x) = \Tv^{+\eps(x)}(\set{\Tx_{i,1}, ..., \Tx_{i, x_i p_i / \eps(x)}}_{i \in [n]})$$
    $$ v^{+}(x) = \Tv^{+\eps(x)}\left(\set{\bone_{p_i / \eps(x)}^{x_i p_i / \eps(x)}}_{i \in [n]}\right)$$
    where $\eps(x) \in 1 / \Z_+$ is the largest number divides all $\set{x_i}_{i \in [n]}$. Then, for every $x \in \Q_{[0,1]}^n \to \R_+$,
    $$ v^{+}(x) = v(x)$$
\end{lemma}
\begin{proof}
    One may think $x$ into $\eps(x)$ small pieces. Then, $v^+(x) = v(x)$ follows from simple rearranging. For completeness, we give the following calculation. For $x \in \Q_{[0,1]}^n$, since $\eps(x) \in 1 / \Z_+$ is the largest number divides all $\set{x_i}_{i \in [n]}$, we have  
    \begin{align*}
        v(x) &= - \sum_{i < i' \in [n]} x_i x_{i'} \min\{p_i w_{i'}, p_{i'} w_i\} - \frac{1}{2} \sum_{i \in [n]} x_i x_i w_i p_i + \sum_{i \in [n]} (M - \frac{1}{2} w_i p_i) x_i \\
        &= - \sum_{i < i' \in [n]} \sum_{j \in [x_i p_i / \eps(x)]}\frac{\eps(x)}{p_i} \sum_{j' \in [x_{i'} p_{i'} / \eps(x)]}\frac{\eps(x)}{p_{i'}} \min\{p_i w_{i'}, p_{i'} w_i\} \\
        &- \frac{1}{2} \sum_{i \in [n]} \left(\sum_{j \in [x_i p_i / \eps(x)]}\frac{\eps(x)}{p_i}\right)^2 w_i p_i + \sum_{i \in [n]} (M - \frac{1}{2} w_i p_i) \sum_{j \in [x_i p_i / \eps(x)]}\frac{\eps(x)}{p_i} \\
        &= - \eps(x)^2 \sum_{i < i' \in [n]} \sum_{j \in [x_i p_i / \eps(x)]} 1 \sum_{j' \in [x_{i'} p_{i'} / \eps(x)]} 1 \cdot \min\{\frac{w_{i}}{p_i}, \frac{w_{i'}}{p_{i'}}\} \\
        &- \frac{1}{2} \eps(x)^2 \sum_{i \in [n]} \left(\sum_{j \in [x_i p_i / \eps(x)]} 1\right)^2 \frac{w_i}{p_i} + \eps(x) \sum_{i \in [n]} (\frac{M}{p_i} - \frac{1}{2} w_i) \sum_{j \in [x_i p_i / \eps(x)]} 1 \\
        &= \Tv^{+\eps(x)}\left(\set{\bone_{p_i / \eps(x)}^{x_i p_i / \eps(x)}}_{i \in [n]}\right) = v^+(x)
    \end{align*}
\end{proof}

\begin{lemma}
    \label{lem:v-eps-submodular}
    For any $\eps \in 1 / \Z_+$, let $v^{+\eps}(x) = \Tv^{+\eps}\left(\set{\bone_{p_i / \eps(x)}^{x_i p_i / \eps(x)}}_{i \in [n]} \right)$ for $x \in \set{\eps \Z_+ \leq 1}^n$. Then, the dual profit is submodular, i.e., $\pi^{+\eps}(q) = \max_{x \in \set{\eps \Z_+ \leq 1}^n} v^{+\eps}(x) - q \cdot x$ for $q \in \R^n$.
\end{lemma}
\begin{proof}
    Notice that $\Tv^{+\eps}$ is gross substitutes. Then, its dual profit $\tilde \pi^{+\eps}$ is submodular. Consider any $q \in \R^n$. We have
    \begin{align*}
        \pi^{+\eps}(q) &= \max_{x \in \set{\eps \Z_+ \leq 1}^n} v^{+\eps}(x) - q \cdot x \\
        &= \max_{x \in \set{\eps \Z_+\leq 1}^n} \Tv^{+\eps}\left(\set{\bone_{p_i / \eps}^{x_i p_i / \eps}}_{i \in [n]}\right) - \left( \set{\underbrace{q_i \eps / p_i, ..., q_i \eps / p_i}_{\text{divides}\ q_i \ \text{into} \ p_i / \eps\ \text{parts}}}_{i \in [n]} \right) \cdot \set{\bone_{p_i / \eps}^{x_i p_i / \eps}}_{i \in [n]} \\
        &= \tilde \pi^{+\eps} (\set{q_i \eps / p_i, ..., q_i \eps / p_i}_{i \in [n]})
    \end{align*}
    Thus, the lemma follows from the submodularity of $\tilde \pi^{+\eps}$.
\end{proof}

\begin{lemma}
    \label{lem:v-weighted-nonclair--dualprofit-submodular}
    The dual profit of $v^+$ is submodular, i.e., $\pi^+(p) = \max_{x \in \Q_{[0,1]}^n} v^+(x) - p \cdot x$ for $p \in \R^n$.
\end{lemma}
\begin{proof}
    Suppose that $\pi^+$ is not submodular. Then, there are $p, q \in \R^n$ that violate the submodularity such that
    $$ \pi^+(p) + \pi^+(q) < \pi^+(p \vee q) + \pi^+(p \wedge q) $$
    Consider $\pi^+(p)$. Let $\eps_p \in 1 / \Z_+$ be the parameter such that 
   % $$ \pi^+(q) = \max_{\Tx \in \set{0,1}^{\sum_{i\in[n]} p_i/\eps_q}} v^{\eps_q}(\Tx) - q \cdot \left(\set{\sum_{j\in[p_i / \eps_q]} \Tx_{i,j}}_{i\in[n]} \right)$$
    $$ \pi^+(p) = \pi^{+\eps_p}(p)$$
    Then, let $\eps'$ be the largest number in $1 / \Z_+$ divides $\eps_p, \eps_{q}, \eps_{p \wedge q}, \eps_{p \vee q}$. Thus, $\pi^{+\eps'}(p) \geq \pi^{+\eps_p}(p)$, $\pi^{+\eps'}(q) \geq \pi^{+\eps_q}(q)$, $\pi^{+\eps'}(p \vee q) \geq \pi^{+\eps_{p \vee q}}(p \vee q)$ and $\pi^{+\eps'}(p \wedge q) \geq \pi^{+\eps_{p \wedge q}}(p \wedge q)$. Due to the optimality, we have 
    $$ \pi^{+\eps'}(p) + \pi^{+\eps'}(q) < \pi^{+\eps'}(p \vee q) + \pi^{+\eps'}(p \wedge q) $$
    Therefore, the lemma holds true from the submodularity of $\pi^{+\eps'}$ due to Lemma~\ref{lem:v-eps-submodular}.
\end{proof}

\begin{lemma}
    $v$ is linear substitutes.
\end{lemma}
\begin{proof}
    Consider its dual profit $\pi(p) = \max_{x \in \R^n} v(x) - p \cdot x$. Suppose that $\pi$ is not submodular. Then, we have $p, q \in \R^n$ that violate the submodularity such that 
    $$ \pi(p) + \pi(q) < \pi(p \vee q) + \pi(p \wedge q) $$
    Let $\Delta$ be the difference of the above inequality.
    Due to the continuity and $v(x) = v^+(x)$ for $x \in \Q_{[0,1]}^n$, for some infinitesimally $\eps' > 0$,  we have $|\pi^{+}(p) - \pi(p)|, |\pi^{+}(q) - \pi(q)|, |\pi^{+}(p \vee q) - \pi(p \vee q)| \ \text{and} \ |\pi^{+}(p \wedge q) - \pi(p \wedge q)|$ are less than $\eps'$. Since $\Delta - 4 \eps' > 0$, we have 
    $$\pi^{+}(p) + \pi^{+}(q) < \pi^{+}(p \vee q) + \pi^{+}(p \wedge q)$$  
    This would contradict the submodularity of $\pi^{+}$ from Lemma~\ref{lem:v-weighted-nonclair--dualprofit-submodular}, and thus we prove the lemma.
\end{proof}
